# Supplementary material for: Convex Relaxations for Pose Graph Optimization with Outliers
Source: arXiv:1801.02112 source file (2018-01-07)
Supplement: Supplementary file 1 [file appendix.tex]

%!TEX root = Special Issue COMPENG2016 - Draft.tex

\appendix

\subsection*{Proof of Proposition~\ref{prop:l2OnPosesPrimal}}
